# Supplementary material for: Learning Latent Events from Network Message Logs
Source: arXiv:1804.03346 source file (2019-07-17)
Supplement: Supplementary file 1 [file supp.tex]

\documentclass{article}

\usepackage[utf8]{inputenc}

\usepackage{enumitem}
\usepackage{caption}
\usepackage{subcaption}
\usepackage{url}
\usepackage{amsmath,amssymb,amsthm,amsfonts}
\usepackage{algorithm}
\usepackage[noend]{algpseudocode}

\usepackage{graphicx}
\usepackage{textcomp}
\usepackage{comment}
\usepackage{dsfont}
\def\BibTeX{{\rm B\kern-.05em{\sc i\kern-.025em b}\kern-.08em
    T\kern-.1667em\lower.7ex\hbox{E}\kern-.125emX}}

\begin{document}
\title{Supplementary material for Learning Latent Events from Network Message Logs}

\maketitle

%\appendices
%\section{Appendix}
\input{appendix.tex}
\bibliographystyle{ieeetr}
\bibliography{myref,ref}
\end{document}
